# Supplementary material for: Leveraging Visemes for Better Visual Speech Representation and Lip Reading
Source: arXiv:2307.10157 source file (2023-07-19)
Supplement: Supplementary file 1 [file appendices.tex]

\section{Proof of the First Zonklar Equation}
Appendix one text goes here.

% you can choose not to have a title for an appendix
% if you want by leaving the argument blank
\section{}
Appendix two text goes here.
